# Supplementary material for: Nano-silica based Aqueous Colloidal Gels as Eco-friendly Thixotropic Lubricant
Source: arXiv:2506.16249 ancillary file (2025-06-27)
Supplement: Supplementary file 1 [file Supporting_Information.pdf]

# Supporting Information: Nano-silica based Aqueous Colloidal Gels as Eco-friendly Thixotropic Lubricant

Arun Kumar[1], Vivek Kumar[2], Yogesh M. Joshi[2**], and Manjesh Kumar Singh[1*]

[1]Department of Mechanical Engineering, Indian Institute of Technology Kanpur, Kanpur-208016, Uttar Pradesh, India.
[2]Department of Chemical Engineering, Indian Institute of Technology Kanpur, Kanpur-208016, Uttar Pradesh, India.
**manjesh@iitk.ac.in*
*arunkumar20@iitk.ac.in; kvivek@iitk.ac.in; **joshi@iitk.ac.in*

## S1 Tribological tests

The experimental setup's fundamental configuration is illustrated schematically in Figure S1(a). The testing configuration utilized a solid ball as the pin, thus adopting a ball-on-disc arrangement, as depicted in Figure S1(b).

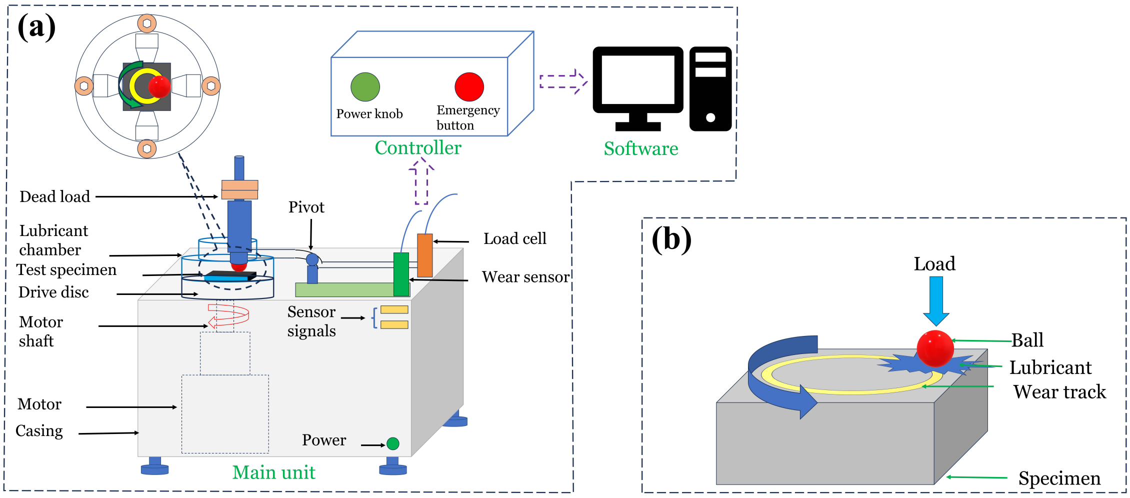


Figure S1: Schematic of (a) experimental set-up for tribological tests and (b) Ball-on-disc assembly associated with the set-up. The normal force applied to the tribopair was exerted by dead weights. The frictional force was measured by a precise load cell when the arm carrying the ball holder made contact with it at its trailing edge. Both the ball and disc were kept within a lubricant cup. Before each test, they were thoroughly cleaned with ethanol. To minimize experimental errors, the arm carrying the ball holder was maintained in a horizontal position.

# S2 Effect of load and speed on the tribological performance

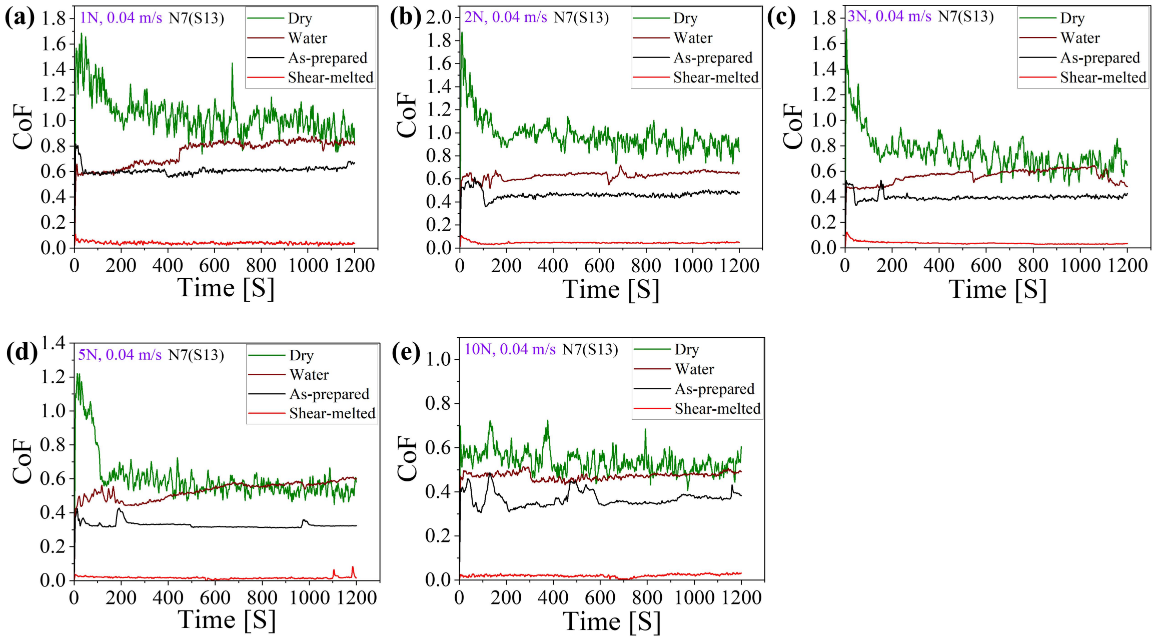


Figure S2: CoF variation at a sliding speed of 0.04 m/s under different normal loads: (a) 1 N, (b) 2 N, (c) 3 N, (d) 5 N, and (e) 10 N, using N7(S13) lubricant.

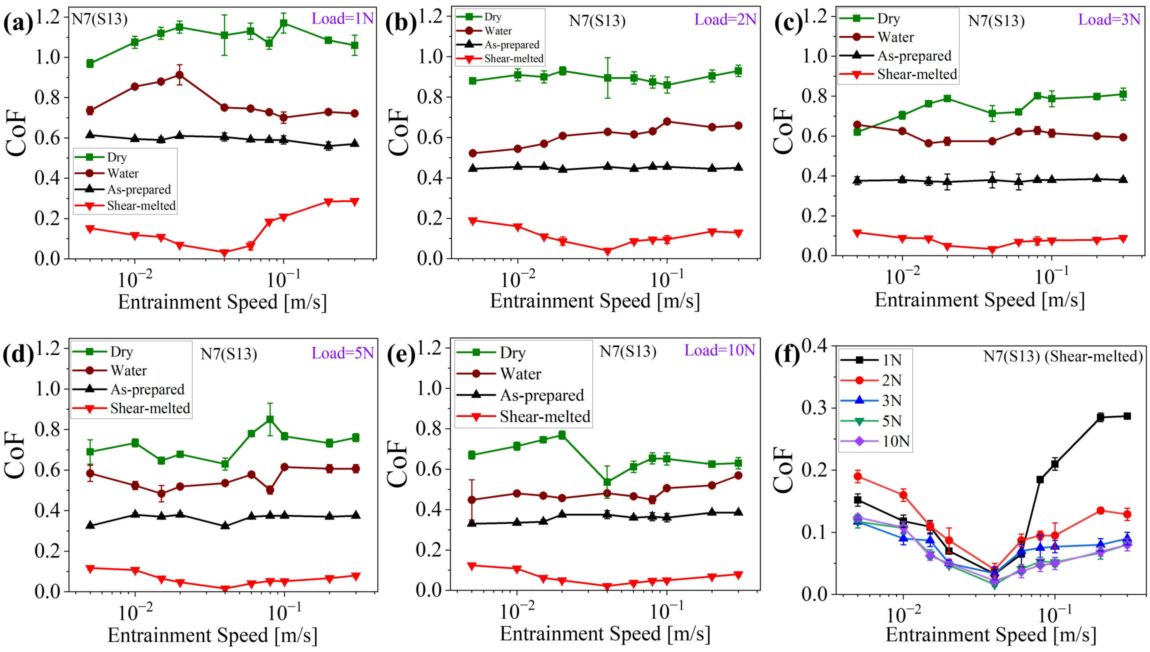


Figure S3: Change in CoF with entrainment speed at load of (a) 1N (b) 2N (c) 3N (d) 5N and (e) 10N (f) CoF variation with entrainment speed at shear-melted condition for different loads. Tests were conducted with N7(S13) lubricant.

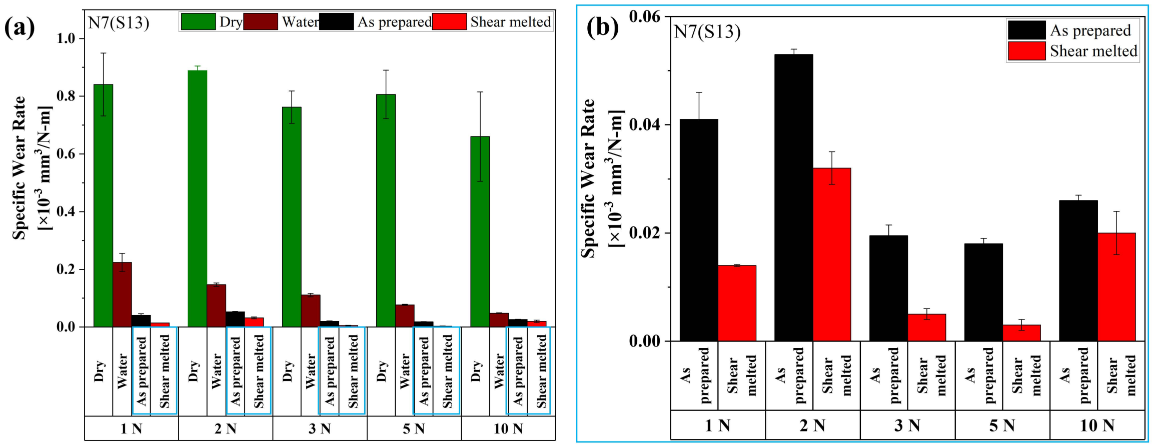


Figure S4: (a) Specific wear rate of disc at sliding speed of 0.04 m/s and at load of 1N, 2N, 3N, 5N and 10N (b) Enlarged view of specific wear rate at as-prepared and shear-melted conditions. Tests were conducted with N7(S13) lubricant.

# S3 Materials and methods

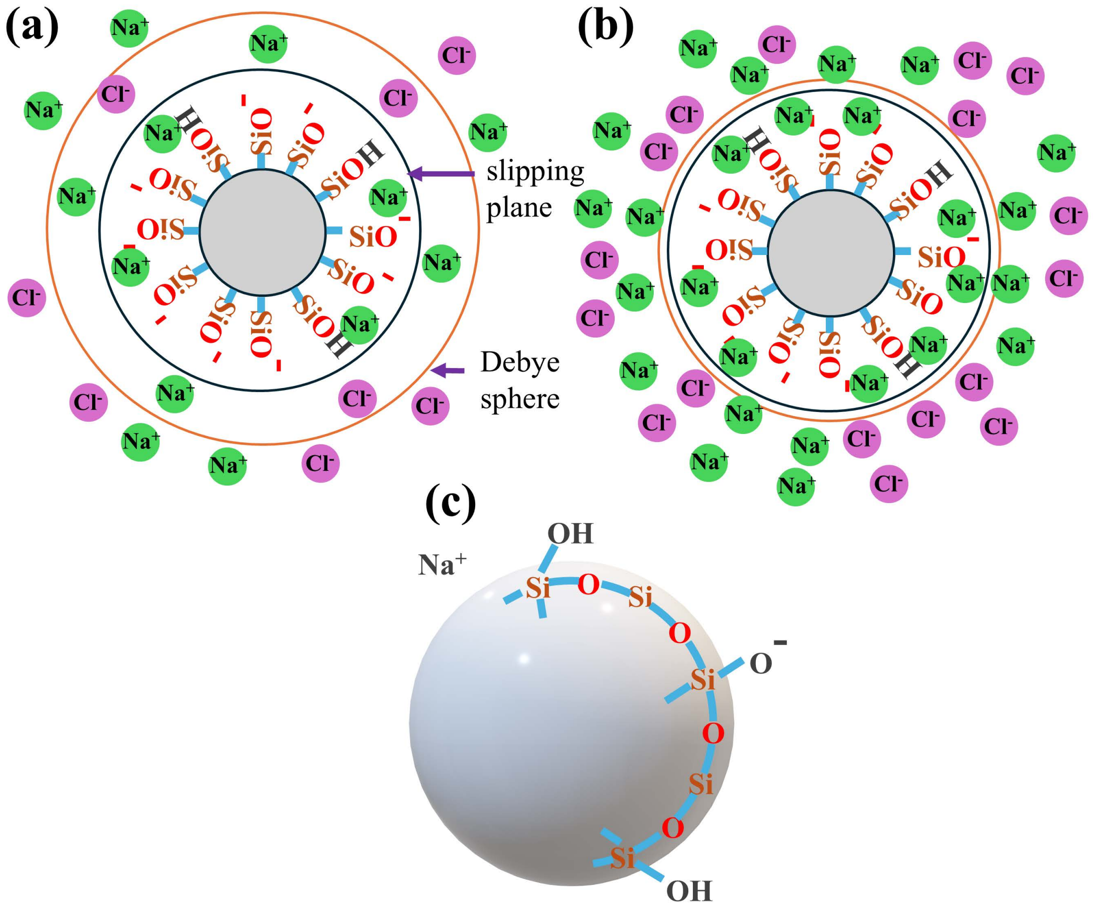


Figure S5: Illustration of ion interaction with a silica surface and its effect on the Debye length (a) at low ion concentration, few cations adsorb onto the silica surface, resulting in a relatively longer Debye length. (b) at higher ion concentration, more cations adsorb onto the silica surface, reducing the Debye length as indicated by the smaller Debye sphere. In both scenarios, the slipping plane, which marks the boundary between the stern layer and the diffuse layer, remains unchanged. (c) Illustration of single particle of Sodium stabilized colloidal silica

# S4 Gelation Kinetics

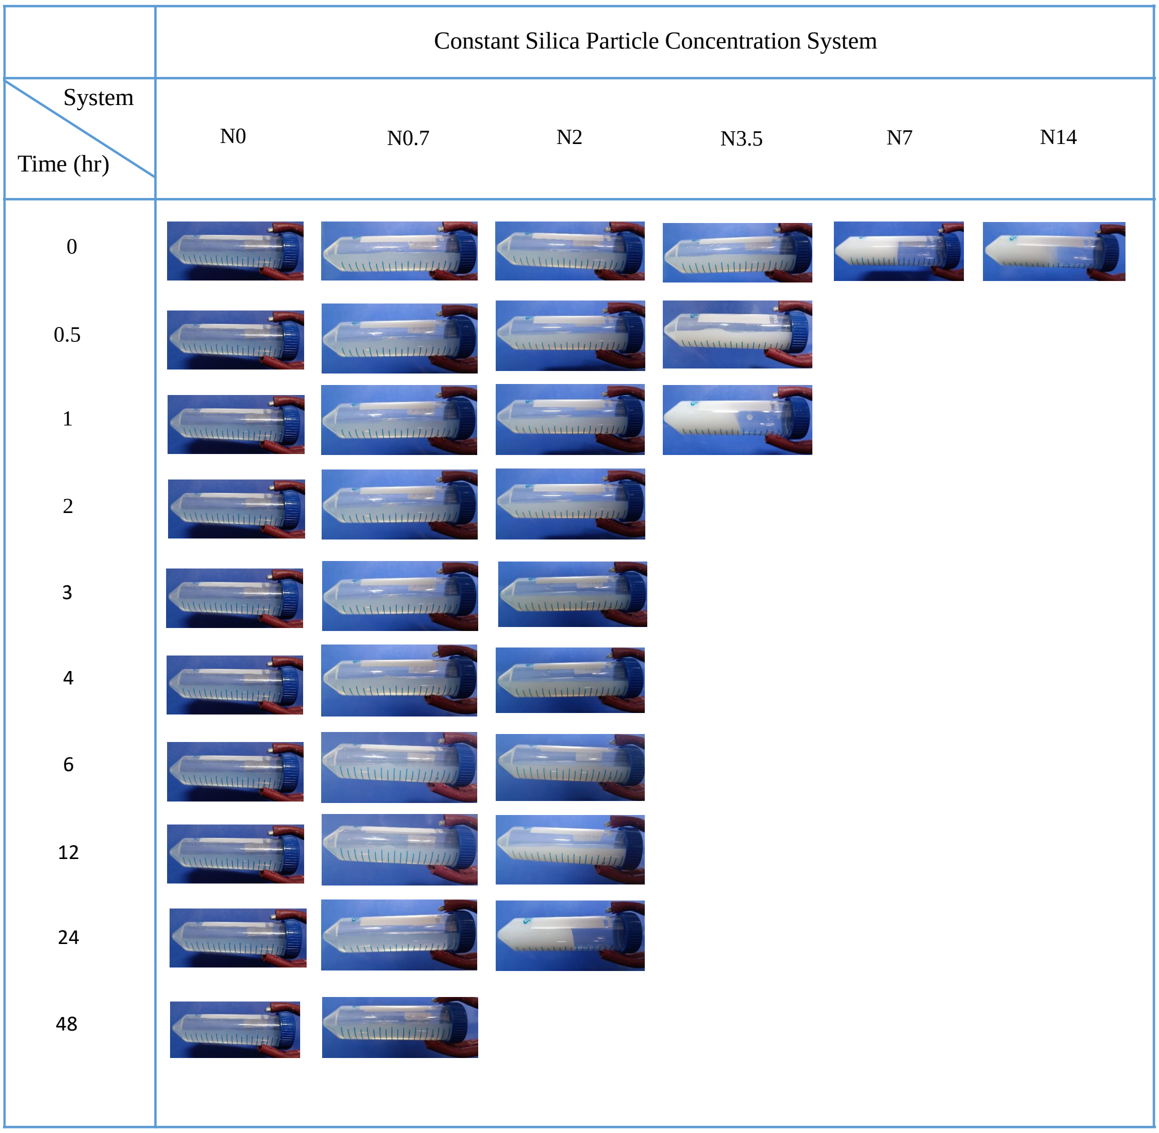


Figure S6: The snapshots of the constant silica particle (13 wt.%) concentration system with the varying concentration of the NaCl salt starting from 0 to 48 hrs.

| | Constant NaCl Concentration System | | | | |
|---|---|---|---|---|---|
| System / Time (hr) | S3 | S7.5 | S13 | S17.5 | S20 |
| 0 | 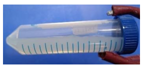 | 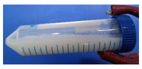 | 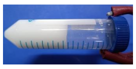 | 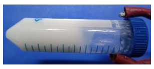 | 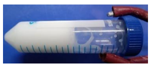 |
| 0.5 | 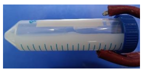 | 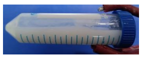 | | | |
| 1 | 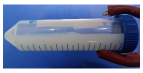 | 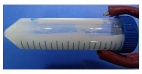 | | | |
| 2 | 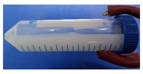 | 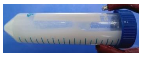 | | | |
| 3 | 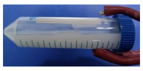 | 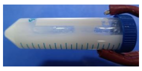 | | | |
| 4 | 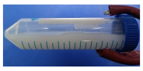 | 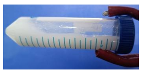 | | | |
| 6 | 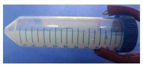 | 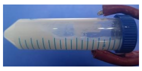 | | | |
| 12 | 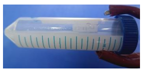 | 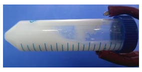 | | | |
| 24 | 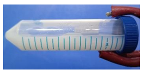 | 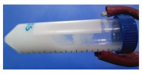 | | | |
| 48 | 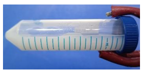 | 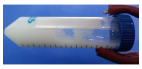 | | | |

Figure S7: The snapshots of the constant NaCl (7 wt.%) concentration system with the varying concentration of silica particles starting from 0 to 48 hrs.

# S5 Rheological study

## S5.1 Viscosity vs. shear rate

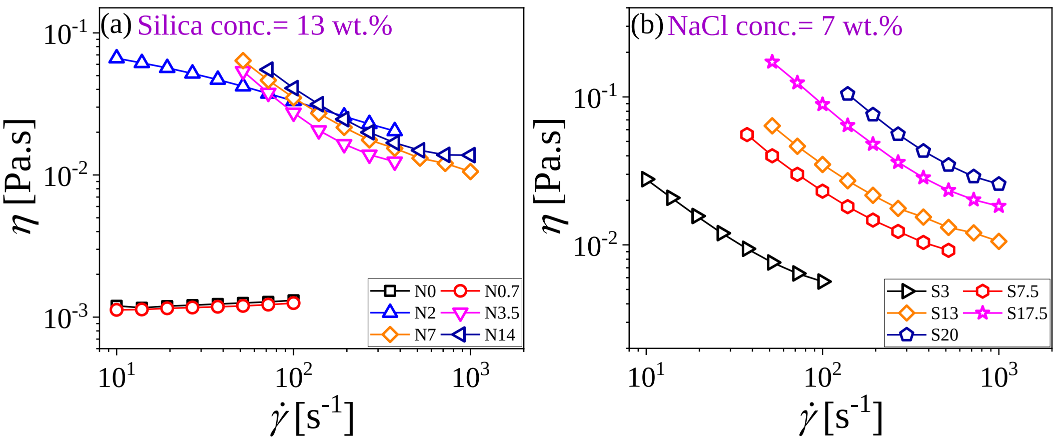


Figure S8: Viscosity is plotted against the shear rate for (a) constant silica concentration and (b) constant NaCl concentration systems. In (a), the N0 and N0.7 systems show the Newtonian behavior, whereas other systems show the shear thinning behavior due to structural breakdown at a higher shear rate. In (b), all the systems show shear-thinning behavior.

## S5.2 Time aging-time superposition

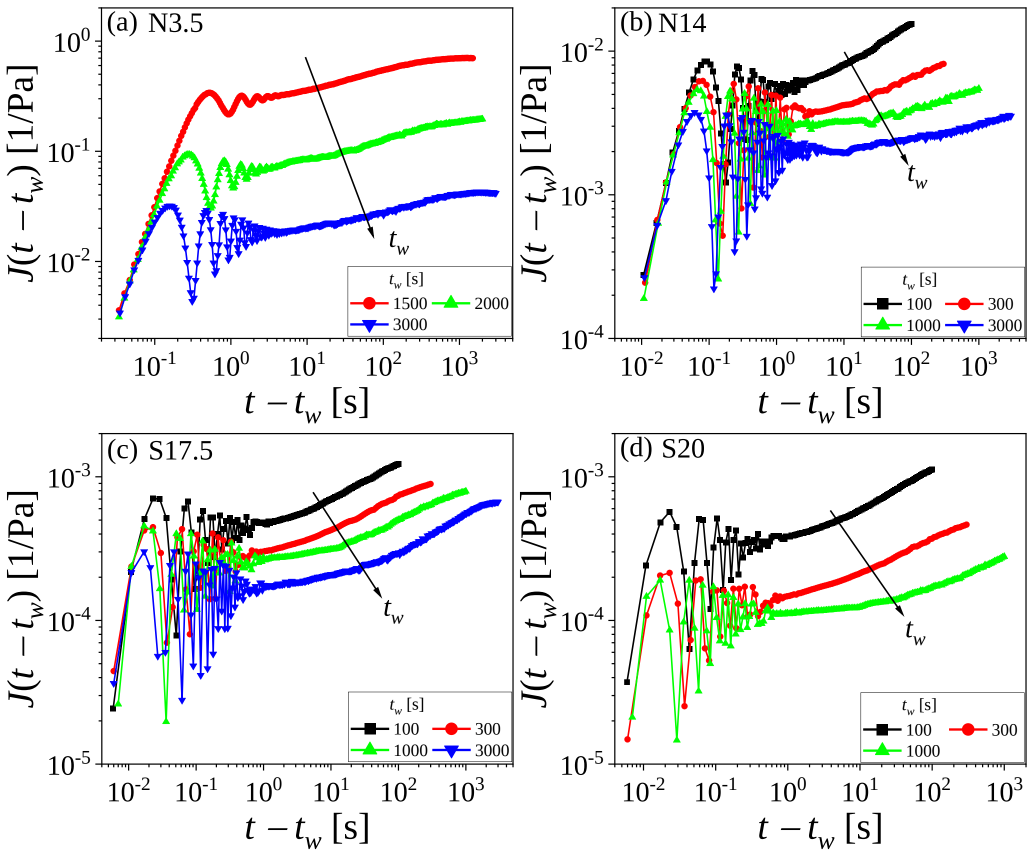


Figure S9: The creep compliance curves are plotted as a function of creep time for (a) N3.5, (b) N14, (c) S17.5, and (d) S20 systems. The stress applied to the different systems during the creep experiments is 0.1 Pa (N3.5), 0.2 Pa (N14), 2 Pa (S17.5), and 4 Pa (S20), respectively. The arrow is the guide to the eye for increasing magnitude of waiting time ($t_w$). As the $t_w$ increases, the creep compliance curves shift vertically downward due to aging. Different symbols are assigned for the creep experiments done at different $t_w$ and are given in the legend.

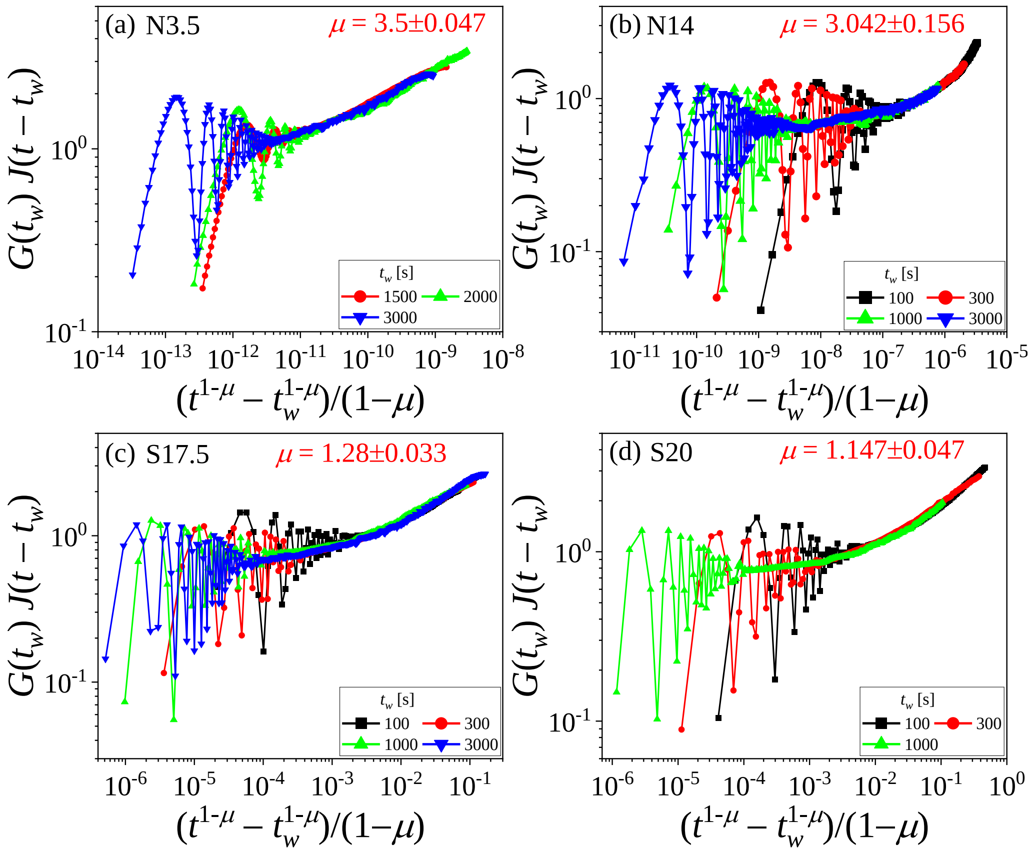


Figure S10: The scaled creep compliance curves ($G(t_w)J(t-t_w)$) is plotted against the effective time ($(t^{1-\mu}-t_w^{1-\mu})/(1-\mu)$) for (a) N3.5, (b) N14, (c) S17.5, and (d) S20. All the creep curves superimpose on each other for the unique value of $\mu$. The power law coefficient ($\mu$) for each system is given in the inset of the respective plot.

# S6 Surface characterization of unworn disc

To measure surface roughness, five randomly selected regions, each approximately $1.45 \times 1.9$ mm$^2$ in size, were examined for each specimen. The root mean square (RMS) roughness, an essential parameter for measuring surface deviations, was used as the main metric for roughness characterization. The RMS roughness ($R_q$) values in nanometers (nm), along with their standard deviations, were recorded for specimens prior to friction tests. Analysis of the data indicates that the average RMS roughness for specimens tested under specific conditions across different lubrication scenarios is $17.664 \pm 3.013$ nm. In boundary lubrication scenarios, the initial roughness characteristics are highly significant. When the lubricant film thickness is minimal, RMS roughness values can significantly affect the degree of direct contact between mating surfaces. Care was taken to maintain a consistent surface condition for all specimens during tribological testing to ensure the reliability of the results.

# S7 Evaluation of lubrication regime

Establishing the lubrication regime is essential for understanding the system, as the non-Newtonian flow behavior of grease-like semi-solid lubricants complicates their use in machine elements [1, 2]. In elastohydrodynamic lubrication (EHL), film thickness is determined by the lubricant's rheological behavior in the contact inlet, where shear rates are extremely high. Researchers often use various models like Herschel–Bulkley (HB) [3, 4, 5] to describe grease flow at low to moderate shear rates ($\leq 10^4$ s$^{-1}$), assuming they remain valid at higher shear rates ($\geq 10^6$ s$^{-1}$). However, at such high shear rates, grease tends to behave like a Newtonian fluid [6], making HB models based on low-shear data unreliable for predicting lubrication performance [6]. Predicting grease behavior under lubrication is more challenging than for Newtonian oils [7]. Despite its wide use, classical EHL theory is inadequate for estimating film thickness in grease-lubricated systems [8].

Isoviscous-elastic hydrodynamic lubrication, or "soft-EHL," [9, 10] occurs when non-conforming surfaces deform elastically under contact pressure, or the pressure is too low to significantly increase lubricant viscosity at inlet. Common with low pressure-viscosity lubricants like water [11], film thickness in such cases depends more on the elastic properties of the surfaces than on the lubricant's viscosity. These lubricants often have complex, highly non-Newtonian behavior [12], including shear thinning, viscoelasticity, and yield stress. The Hamrock and Dowson equation is most commonly used to describe this regime [13].

$$h_m \approx 2.8 R'^{0.77} (\eta U)^{0.65} (W)^{-0.21} (E')^{-0.44} \tag{S1}$$

$$\lambda = \frac{h_m}{R_q} \tag{S2}$$

$$R_q = \sqrt{R_{ball}^2 + R_{flat}^2} \tag{S3}$$

Here $h_m$ is film thickness, $U$ is sliding speed, $W$ is applied load, $\eta$ is lubricant viscosity, $R^{'}$ is ball radius and $E^{'}$ is reduced elastic modulus. $E^{'}$ is given by $2/E^{'} = (1 - {\nu_1}^2)/E_1 + (1 - {\nu_2}^2)/E_2$. $\nu$ and $E$ are Poisson's ratio and Elastic modulus of two bodies in contact. Since no accurate model exists for film thickness with non-Newtonian lubricants, we use Equation S1, assuming the lubricant's viscosity at a high shear rate, i.e., $10^3$ $s^{-1}$. The lubrication regime is estimated using Equation S2, where $\lambda$ is the ratio of theoretical minimum film thickness $h_m$ and combined surface roughness ($R_q$) of the contacting surfaces. A consistent $\lambda < 1$ indicates boundary lubrication.

# S8 Friction results

Figure S11 (a) shows the friction behavior of aqueous NaCl solutions with varying NaCl concentrations. The friction behavior closely resembles that of dry and pure water conditions, yielding CoF values of 0.54±0.03, 0.53±0.03, 0.52±0.005, 0.51±0.01 and 0.46±0.007 for W0.7, W2, W3.5, W7, and W14, respectively. These results indicate that aqueous NaCl solutions alone are not effective lubricants under the given test conditions. Figure S11 (b) and (c) shows the variation of CoF with test duration for as-prepared and shear-melted lubricants with varying NaCl concentration, respectively. Large fluctuations in the CoF curve are evident for dry sliding and water-lubricated contacts, even after a running-in period of approximately 100s, due to ineffective lubrication and irregular asperity engagement. In contrast, all lubricant formulations exhibited smooth and stable CoF from the beginning of sliding, except for minor fluctuations in N14, indicating an effective boundary lubrication layer (Figure S11 (b)).

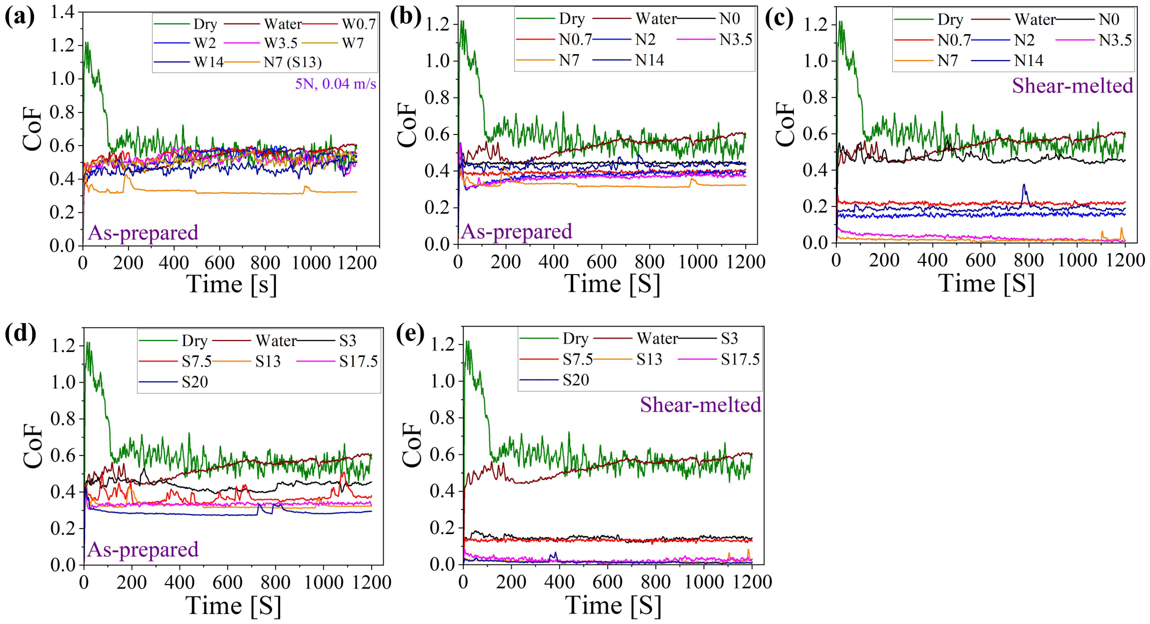


Figure S11: (a) CoF curves for varying NaCl concentrations in water (W0.7 to W14 denote NaCl concentration in wt.%). Variation of CoF over time for lubricants with varying NaCl concentrations and fixed silica concentration of 13 wt.% in (b) as-prepared state (c) shear-melted state. Variation of CoF over time for lubricants with different silica concentrations and fixed NaCl concentration of 7 wt.% in (d) as-prepared state and (e) shear-melted state. Tests were conducted at 5 N and 0.04 m/s.

For shear-melted lubrication (Figure S11 (c)), N0 showed a high fluctuation friction curve due to the absence of gel formation. All other lubricant formulations showed uniform and stable CoF curves. N3.5 and N7 performed similarly for up to 800s, with N7 achieving super-low friction initially, but both converged afterward, suggesting that either formulation is suitable for long duration sliding. This indicates the formation of a thin, protective tribolayer that reduces friction. Further details are discussed in the worn surface analysis section of the main manuscript.

Figure S11 (d) and (e) discusses the variation of CoF with test duration for as-prepared lubricants with varying silica concentration. At low silica concentrations (S3 and S7.5), unstable and high fluctuations are visible in the CoF curve, unlike the stable curves shown by S13, S17.5, and S20 (Figure S11 (d)). However, this phenomenon of CoF fluctuations is not observed in shear-melted lubricants. Additionally, the friction curves of S13, S17.5, and S20 overlap for most of the test duration, maintaining

stable friction coefficient (Figure S11 (e)).

# S9 Specific wear rate calculation (SWR)

Wear volume ($mm^3$) of ball ($V_b$) and disc ($V_d$), is estimated using the ISO 18535:2016 [14] as reported in the main manuscript. As per standard, both the test surface and counterface lose material during the pin-on-disc test. The pin (ball in our study) is assumed to develop a flat end, while the disc shows an approximately circular wear scar. Diameters $A$ and $B$ on the ball, with $A$ being smaller, are measured perpendicularly (Fig. S12(a)), and the cross-sectional areas ($mm^2$) of the wear track are measured at four places (P1-P4) spaced at 90° apart (Fig. S12(b)).

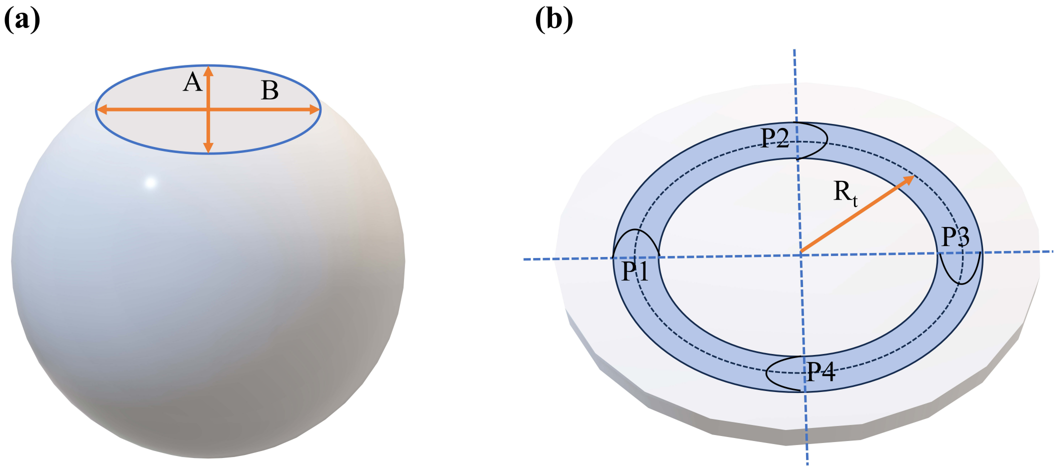


Figure S12: Schematic of (a) wear scar (b) wear track on disc

The wear volume $V_{\mathrm{bISO}}$ and the specific wear rate $W_{\mathrm{sb}}$ ($mm^3$/N-m) of the balls are determined by:

$$V_{\mathrm{bISO}} = \frac{\pi A^3 B}{32D} \tag{S4}$$

$$W_{\mathrm{sb}} = \frac{V_b}{F_n l} \tag{S5}$$

where $D$, $F_n$ and $l$ denote ball diameter (mm), normal load (N), and sliding distance (m) respectively. The same quantities for disc can be evaluated as:

$$V_{\mathrm{dISO}} = \frac{\pi R_t \left(S1 + S2 + S3 + S4\right)}{2} \tag{S6}$$

$$W_{\text{sd}} = \frac{V_d}{F_n l} \tag{S7}$$

$V_{\text{dISO}}$ and $R_t$ and $W_{\text{sd}}$ represents volume of disc wear in $\text{mm}^3$, radius of the wear track in mm and SWR of the disc respectively. The wear track's cross-sectional profile was measured at four points, as shown in Figure S12(b). The 2D and 3D image of the worn segment is presented in Figures S13(a) and (b) for illustration, with a representative 2D profile shown in Figure S13(c). Cross-sectional areas at these four locations, were calculated using trapezoidal integration in Origin 2022b.

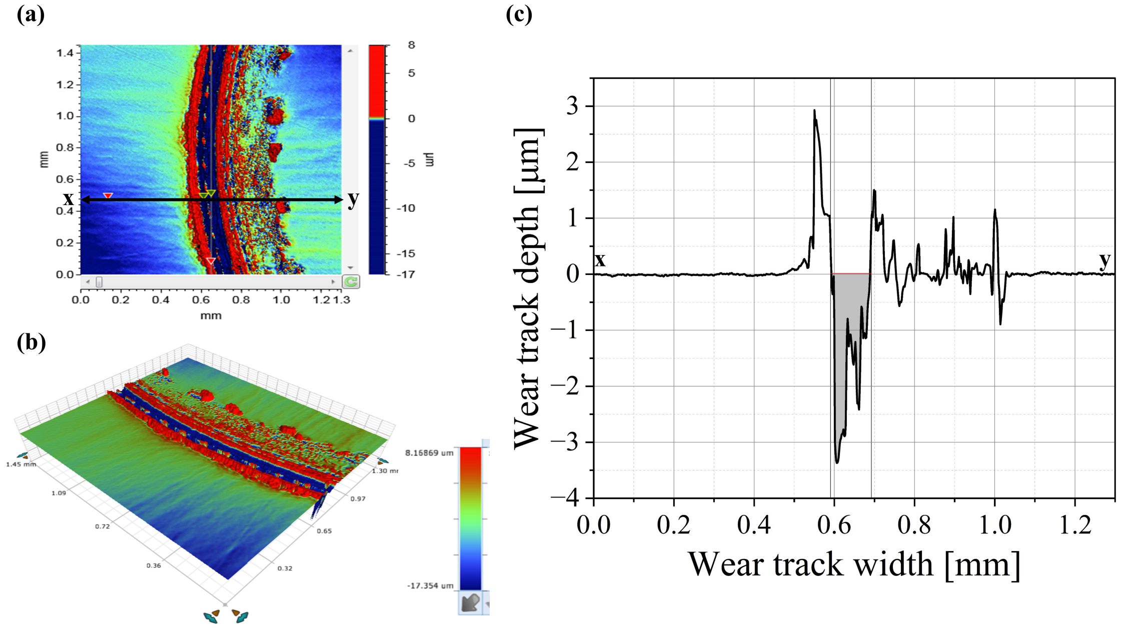


Figure S13: (a) 2D (b) 3D image of a worn-out track segment of disc lubricated with N7 lubricant in as-prepared lubrication method. Images were obtained using 3D optical profilometer (c) cross-sectional profile of wear track along x-y

The wear volume was calculated by multiplying the average of four measured cross-sectional areas with the wear track's circumference (equation S6). The disc's SWR was then determined using equation S7.

# S10 Worn surface analysis

Figure S14 shows the worn disc surface after dry sliding and water-lubricated sliding. In dry sliding (Figure S14 (a)), the worn surface shows craters with fragmented debris

due to direct contact between sliding surfaces. High friction causes localized adhesion and material transfer. Localized heating leads to micro-welding at contact points, which break during sliding, forming debris and craters. In water-lubricated sliding (Figure S14 (b)), the worn surface has deep grooves, silica particles, wear debris, and foreign carbon particles. EDS analysis confirms the presence of silica (Si and O) (Figure S14 (i, ii, iii)). Wear debris enters the contact zone resulting in grooves and exacerbate wear. Presence of foreign carbon particles (confirmed by EDS (Figure S14 (iv)) is also observed.

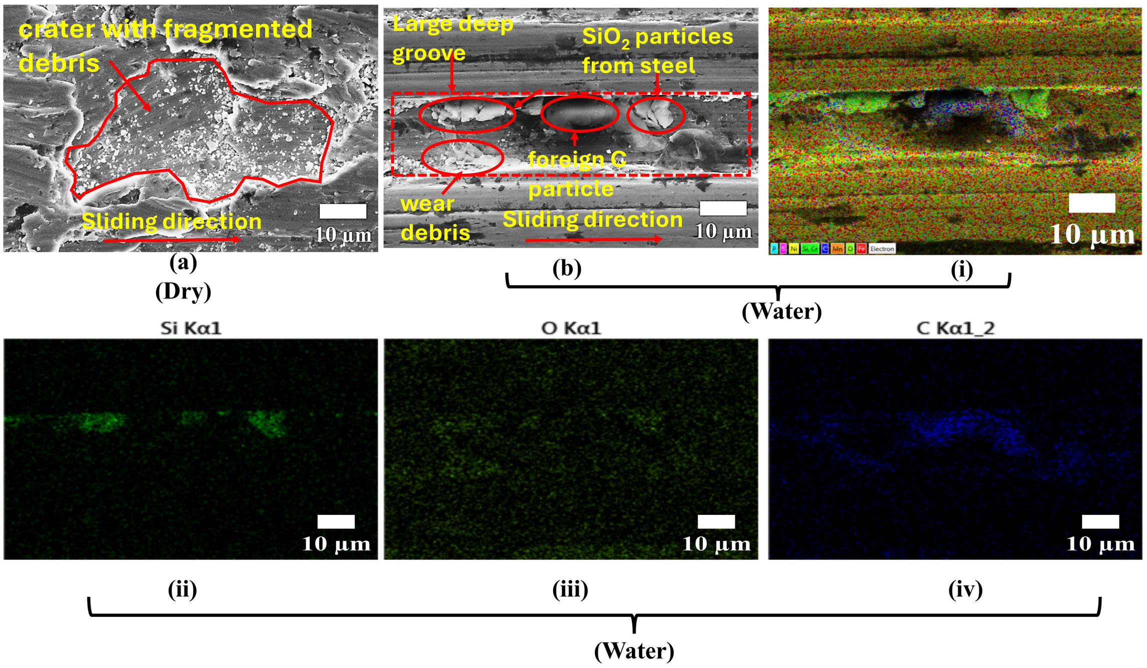


Figure S14: SEM and EDS images of the worn disc surface at dry (a) and water (images b, i, ii, iii, iv) condition.

Figure S15 shows worn disc surface after lubrication with different NaCl concentration i.e., N0.7, N2, N3.5, N14 in as prepared lubrication condition. The worn surface, lubricated with N0.7 (Figure S15 (a)) showed abrasion marks and silica-filled cavities, dominated by abrasive wear. The low NaCl concentration results in a weak gel structure, preventing lubricant film formation. Hard abrasives from sliding debris cause abrasion. Instead of forming tribolayer, silica gel filled cavities confirmed by EDS images (Figure S15 (i, ii, iii)). For N2, the worn surface (Figure S15 (b)) exhibited deep furrows, trapped debris, and parallel grooves. The increased gel strength retains some silica particles within the gel matrix, but it is insufficient to prevent

deep furrowing. Trapped silica particles (confirmed by Figure S15 (iv, v, vi)) show the gel's attempt to mend the surface but ineffective protection against friction and wear.

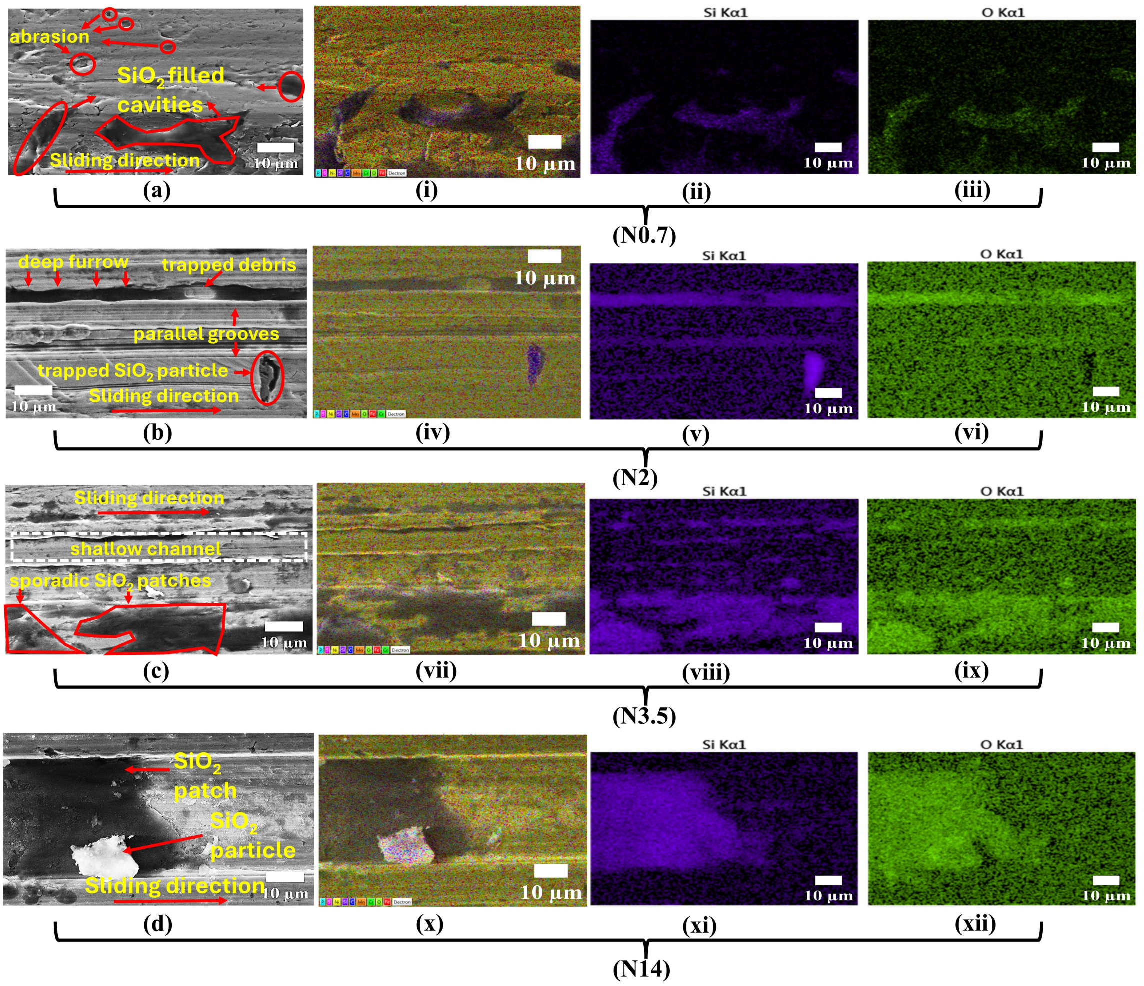


Figure S15: SEM and EDS images of the worn disc surface at different NaCl concentrations: N0.7 (images a, i, ii, iii), N2 (images b, iv, v, vi), N3.5 Images (c, vii, viii, ix) and N14 (d, x, xi, xii) for as-prepared lubricant.

In N3.5 (Figure S15 (c)), the surface showed shallow channels and sporadic silica patches. With higher NaCl concentration, the gel becomes stronger, better holding silica particles, resulting in shallower wear channels. The sporadic silica patches (Figure S15 (vii, viii, ix)) suggest partial surface protection from abrasive wear. For N14, the surface (Figure S15 (d)) exhibited large, partial, and discontinuous silica

patches with chunks of silica particles. The highest NaCl concentration maximizes gel strength, forming large silica patches that partially protect the surface. However, discontinuous patches and silica chunks (Figure S15 (x, xi, xii)) suggest the gel can trap larger particles but may fail to uniformly cover the surface, leading to mixed wear mechanisms.

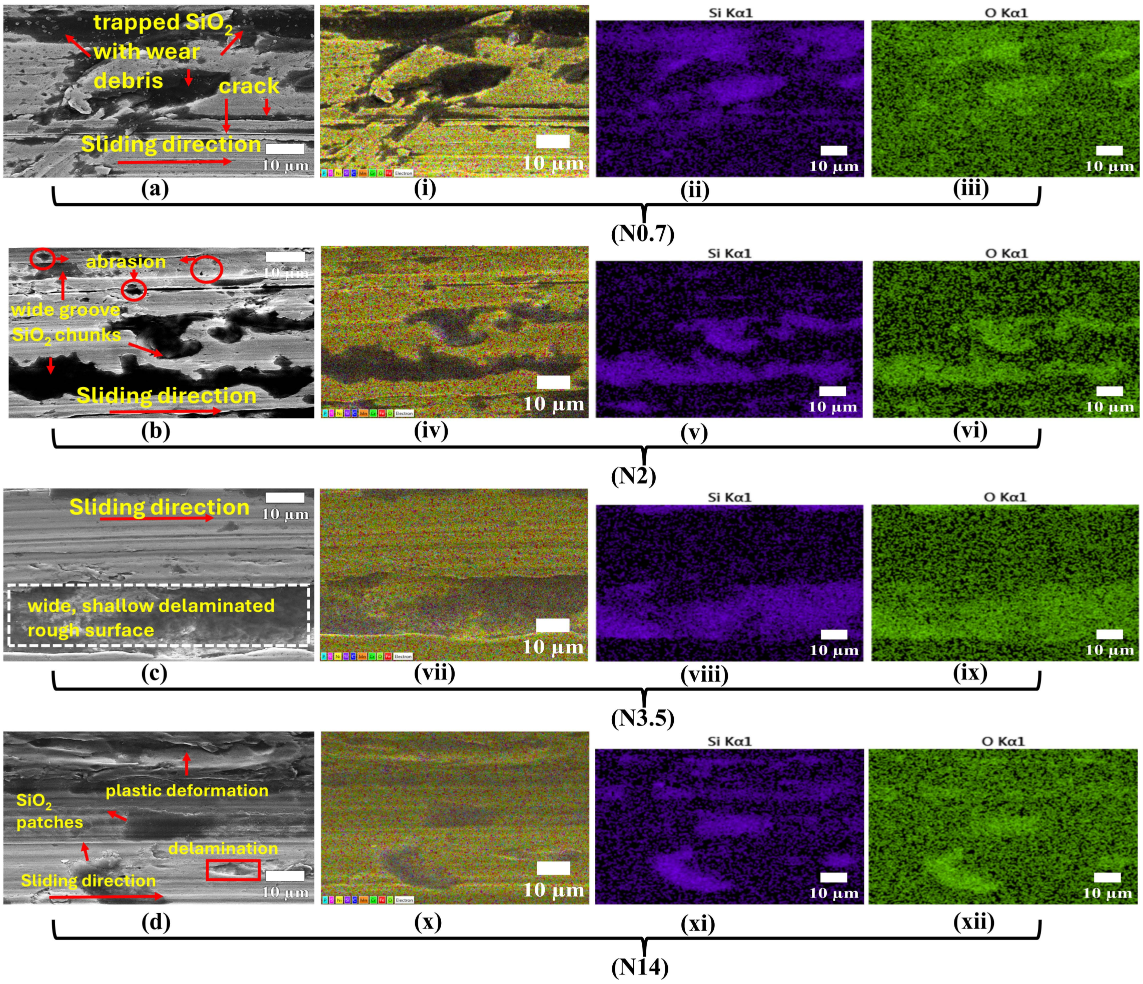


Figure S16: SEM and EDS images of the worn disc surface at different NaCl concentrations: N0.7 (images a, i, ii, iii), N2 (images b, iv, v, vi), N3.5 Images (c, vii, viii, ix) and N14 (d, x, xi, xii) for shear-melted lubricant.

Figure S16 illustrates worn disc surfaces lubricated under shear-melted conditions with varying NaCl concentrations (N0.7, N2, N3.5, N14). At N0.7 concentration (Figure S16 (a, i, ii, iii)), the surface shows trapped silica particles, wear debris, and

visible cracks along the sliding direction, reflecting the gel's minimal structural integrity. This leads to inadequate rebuilding after shear stress and results in poor load carrying capacity. Surface lubricated with N2 concentration (Figure S16 (b, iv, v, vi)) exhibits abrasion marks and wide grooves, indicating significant abrasive wear. Despite the presence of large silica chunks, the gel structure fails to fully reform and cover the entire surface. For N3.5 concentration (Figure S16 (c, vii, viii, ix)) wide, shallow, rough surface due to delamination wear, despite some improvement in gel structure, are visible. Finally, N14 concentration (Figure S16 (d, x, xi, xii)) displays evidence of plastic deformation, including scattered silica patches and delamination, suggesting substantial plastic flow and a combination of plastic deformation and delamination wear.

Figure S17 depicts worn disc surfaces lubricated with varying silica concentrations (S7.5, S17.5) under both as-prepared and shear-melted conditions. The surface lubricated with S7.5 concentration, as shown in Figure S17 (a, i, ii, iii), exhibits desquamation, wear debris, and wide ploughing along the sliding direction. The gel structure attempts to mend the surface irregularities caused by sliding but fails to provide adequate lubrication, resulting in delamination. For S17.5 concentration, silica flocs are trapped in large delaminated regions, indicating that the gel structure tries to cover the surface in chunks rather than forming a continuous layer (Figure S17 (b, iv, v, vi)). In the shear-melted state, the S7.5 lubricated surface, shown in Figure S17 (c, vii, viii, ix), exhibits wide ploughing with visible trapped wear debris and micro ploughing. In contrast, for the S17.5 concentration, a clear intermittent silica tribo layer is visible (Figure S17 (d, x, xi, xii)), providing resistance to wear, but there is still a risk of metal-metal contact occurring in the gaps between this layer.

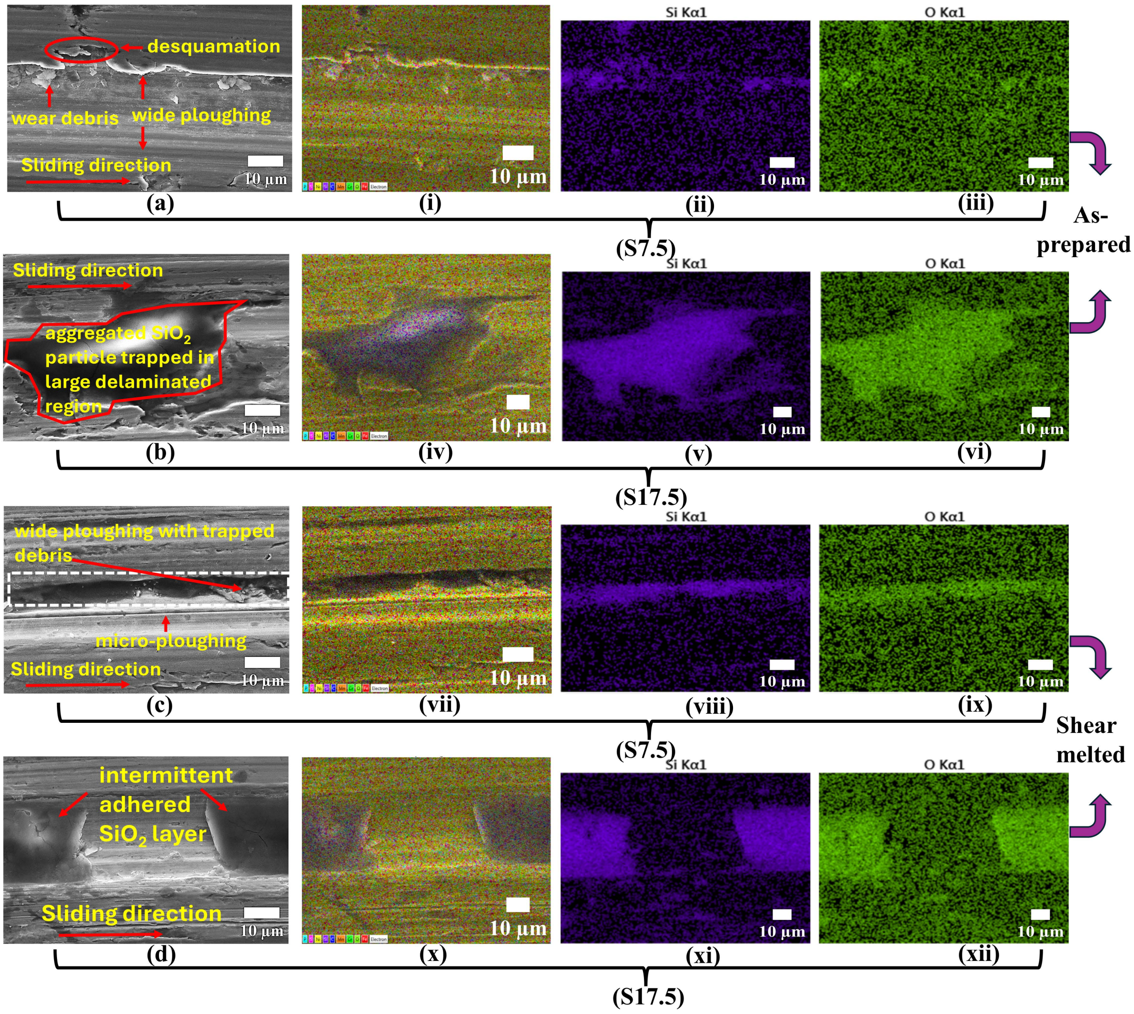


Figure S17: SEM and EDS images of the worn disc surface at different concentrations of silica: S7.5 (images a, i, ii, iii) and S17.5 (images b, iv, v, vi) for the as-prepared lubricant. Images (c, vii, viii, ix) and (d, x, xi, xii) show the worn disc surfaces for S7.5 and S17.5, respectively, for shear-melted lubricant.

# References

[1] L. Paouris, R. Rahmani, S. Theodossiades, H. Rahnejat, G. Hunt, and W. Barton. An Analytical Approach for Prediction of Elastohydrodynamic Friction with Inlet Shear Heating and Starvation. *Tribology Letters*, 64(10):1–18, 10 2016. ISSN 10238883. doi: 10.1007/s11249-016-0740-5.

[2] Yaoguang Zhang, Wenzhong Wang, He Liang, and Ziqiang Zhao. Slip status in lubricated point-contact based on layered oil slip lubrication model. *Tribology International*, 144:1–11, 4 2020. ISSN 0301679X. doi: 10.1016/j.triboint.2019.106104.

[3] J. Echávarri Otero, P. Lafont Morgado, E. Chacón Tanarro, E. De La Guerra Ochoa, A. Díaz Lantada, J. M. Munoz-Guijosa, and J. L. Muñoz Sanz. Analytical model for predicting the friction coefficient in point contacts with thermal elastohydrodynamic lubrication. *Proceedings of the Institution of Mechanical Engineers, Part J: Journal of Engineering Tribology*, 225(4):181–191, 4 2011. ISSN 13506501. doi: 10.1177/1350650111398848.

[4] J. A. Greenwood. Elastohydrodynamic lubrication with herschel-bulkley model greases. *ASLE Transactions*, 15(4):269–277, 1972. ISSN 05698197. doi: 10.1080/05698197208981427.

[5] Jun Cheng. Elastohydrodynamic grease lubrication theory and numerical solution in line contacts. *Tribology Transactions*, 37(4):711–718, 1994. ISSN 1547397X. doi: 10.1080/10402009408983350.

[6] Mohd Mubashshir and Asima Shaukat. The Role of Grease Composition and Rheology in Elastohydrodynamic Lubrication. *Tribology Letters*, 67(104):1–20, 12 2019. ISSN 15732711. doi: 10.1007/s11249-019-1218-z.

[7] P M Cann, B P Williamson, R C Coy, and H A Spikes. The behaviour of greases in elastohydrodynamic contacts I The behaviour of greases in elastohydrodynamic contacts. Technical report, 1992.

[8] J. S. Mérieux, S. Hurley, A. A. Lubrecht, and P. M. Cann. Shear-degradation of grease and base oil availability in starved EHL lubrication. *Tribology Series*, 38: 581–588, 2000. ISSN 01678922. doi: 10.1016/s0167-8922(00)80162-5.

[9] K. Shahrivar, E. M. Ortigosa-Moya, R. Hidalgo-Alvarez, and J. de Vicente. Isoviscous elastohydrodynamic lubrication of inelastic Non-Newtonian fluids. *Tribology International*, 140:1–14, 12 2019. ISSN 0301679X. doi: 10.1016/j.triboint.2019.03.065.

[10] Mongkol Mongkolwongrojn, Khanittha Wongseedakaew, and Francis E. Kennedy. Transient elastohydrodynamic lubrication in artificial knee joint with non-Newtonian fluids. *Tribology International*, 43(5-6):1017–1026, 5 2010. ISSN 0301679X. doi: 10.1016/j.triboint.2009.12.041.

[11] J. de Vicente, J. R. Stokes, and H. A. Spikes. The frictional properties of Newtonian fluids in rolling - Sliding soft-EHL contact. *Tribology Letters*, 20(3-4): 273–286, 12 2005. ISSN 10238883. doi: 10.1007/s11249-005-9067-3.

[12] Abdessamed Nessil, Salah Larbi, Hacene Belhaneche, and Maamar Malki. Journal bearings lubrication aspect analysis using non-newtonian fluids. *Advances in Tribology*, pages 1–9, 2013. ISSN 16875915. doi: 10.1155/2013/212568.

[13] B. J. Hamrock and D. Dowson. Isothermal Elastohydrodynamic Lubrication of Point Contacts: Part III-Fully Flooded Result. *Journal of Tribology*, 99(2): 264–275, 1977. ISSN 15288897. doi: 10.1115/1.3453074.

[14] Irene Pessolano Filos, Raffaella Sesana, Massimiliano Di Biase, and Rocco Lupoi. New abrasive coatings: Abraded volume measurements in ceramic ball production. *Journal of Manufacturing and Materials Processing*, 5(3):1–20, 2021. ISSN 25044494. doi: 10.3390/jmmp5030081.
